# Supplementary material for: Open-Set Recognition: a Good Closed-Set Classifier is All You Need?
Source: arXiv:2110.06207 source file (2022-04-13)
Supplement: Supplementary file 1 [file appendix.tex]

\section{Appendix}

\subsection{Limitations and Ethical Considerations}\label{sec:limitations}

In this paper we have aimed to provide a rigorous and repeatable foundation for OSR research, considering both the baseline method and experimental setting. We show that the baseline can be made competitive with state-of-the-art models for the open-set detection task. However, we also find that the baseline method maps novel categories close to the origin of the deep feature space. This is undesirable behaviour as it limits any further discrimination on these novel instances, with the representation containing little information on the images. Future work could consider how to modify the method such that open-set detection performance is maintained while also allowing for discriminative features of novel categories.

The study of OSR is also of immediate practical concern to the machine learning community. Specifically, it offers an indicator that an object encountered during deployment is unfamiliar. This is important in safety critical settings such as autonomous driving and medical imaging, as well as in accounting for biases in training sets through under-representation of specific characteristics. However, we note that the results shown in this paper are far from optimal, meaning care should still be taken in the practical deployment of these algorithms.  

\subsection{VGG32 Architecture}\label{sec:vgg32}

The model consists of a simple series of nine 3$\times$3 convolution layers, with downsampling occurring through strided convolutions every third layer.

\subsection{Proposed FG}

\subsection{Implementation Details}\label{sec:implementation}

We first tune RandAugment hyper-parameters on each dataset, using validation samples from a single set of `known' classes.
Next, we train the VGG32 backbone for 600 epochs using a cosine annealed learning rate with two warm restarts at 200 and 400 epochs, using a batch size of 128.
We further incorporate learning rate warmup to the optimisation procedure and report single model results (no ensembles) for fair comparison.
We only incorporate label smoothing when training on TinyImageNet, finding it not to be helpful on the other, smaller scale, benchmarks.
We also discard the validation set and train on all available training data, taking the model weights after the final epoch rather than using early stopping (we do not find overfitting to be an issue for the lightweight backbone).
All experiments were carried out on a 12GB GPU (predominantly a NVIDIA Titan X), with experiments taking between two and six hours per class split, depending on dataset size.

\subsection{Discussion: What is a `semantic category'?}\label{sec:discussion}

The discussion of `categories' dates back to Aristotle's canonical work \cite{sep-aristotle-categories}, which has been interpreted in numerous ways but broadly considers categories to refer to intrinsic features of an object \cite{category_definition_petty}. More recently, the psychological literature has suggested categorization is a system to summarise and structure our observations \cite{Rosch1978PrinciplesOC}. The key difference between these definitions is that the former considers semantic systems of classification to be intrinsic to the world, while the latter considers them to be conceptual frameworks imposed by us to better understand the world.

In either case, categorisation systems include a set of invariances within a single category,  as well as a set of `factors of variation' to distinguish between categories. Specifically, different instances within a single category will have a set of features which can be freely varied without the category label changing. In computer vision, this often refers to characteristics such as pose and lighting, but could also refer to more abstract features. Meanwhile, the classification system will also have a (possibly abstract) set of factors of variation to which the category label is sensitive.

The difference between the two definitions is that in Aristotelian categories, these invariances and factors of variation ultimately refer to real-world features, while in the psychological definition they are more likely to map onto functionality for some downstream task of interest to us. In this case, with ambiguity in the precise downstream task, the system of categorization is also subject to uncertainty. This aligns with the ideas in \cite{malisiewicz_cvpr08}, who suggest a more flexible approach to recognition, asking `\textit{what is an object like?}' rather that `\textit{what is an object?}'. This distinction has also been drawn by Mandler \cite{mandler_2000}, who distinguishes `perceptual' and `conceptual' categorization, with the former system referring to concrete perceptions of objects, while the latter is more likely to refer to what an object can \textit{do}.

The psychological view is perhaps more relevant to the machine learning community, being more functional and amenable to being learned from data. In this case, abstract categorization systems such as \{\textit{airplane, automobile, ship, truck}\} are acceptable \emph{if they faithfully map onto downstream tasks}. However, we suggest that generic object recognition datasets, particularly small scale ones, are not designed with downstream tasks in mind but rather to demonstrate that machine learning models are capable of distinguishing between abstract classes. Even if the ultimate downstream task does aim to differentiate abstract classes, we suggest that this would require training with a high number of `known' categories. Thus, while current benchmarks are sufficient for research in closed-set classification, the lack of a clear downstream task (and hence a clear system of categorization) makes them ill-suited for open-set recognition research. Recently, there have indeed been attempts to scale up OoD methods to large-scale datasets ~\cite{RoadyPLOS2020,huang2021mos}.

 Concretely, consider a classifier trained on instances of two household pets:  \{\textit{Labrador (dog), British Shorthair (cat)}\}. The precise underlying system of categorization, abstract or otherwise, is unimportant in the closed-world setting in which the downstream task is precisely defined (it is identical to the training task). However, in the open-world setting, the model must be able to distinguish previously unseen objects, perhaps: \{\textit{Poodle (dog), Sphynx (cat)}\}. In this case, the categorization system becomes important. Does our downstream task ultimately care about individual animal species? In this case, both `Poodle' and `Sphynx' should be identified as `open-set' examples. Or is our model intended to be a `cat / dog' classifier? In which case neither belong to the open-set.

In contrast, in the proposed fine-grained setting, the downstream task is precisely defined by the training task (there is little variance in set of possible downstream tasks when training involves differentiating one hundred bird species). In this way, the classification system is made clear by the training set. Furthermore, many practical computer vision classifiers are deployed in constrained domains with precise class definitions, for instance: person recognition (each person is a class); disease classification (each pathology is a class); vehicle recognition (each vehicle is a class).

In conclusion, though the OSR task with abstract class definitions should not be neglected, we suggest that: (a) OSR with abstract classes requires larger scale datasets with more training classes than the current popular benchmarks; (b) the fine-grained problem presents a more precisely defined problem for academic research; and (c) the new setting is of significant practical interest and presents its own set of challenges.
