# Supplementary material for: Open-Set Recognition: a Good Closed-Set Classifier is All You Need?
Source: arXiv:2110.06207 source file (2022-04-13)
Supplement: Supplementary file 2 [file future_directions_ethical_considerations.tex]

\section{Discussion: Future directions and ethical considerations}

\paragraph{Future directions}
As stated in the main paper, a future development of this work would be designing alternate methods of creating OSR splits of varying difficulty from the FGVC datasets. 
For instance, one could create class splits based on their distance in the feature space of a pre-trained network, similarly to \cite{Cui2019MeasuringDG}.
In our proposed setting, it would be natural to use a network pre-trained on the Places dataset, as we use these weights as initialization for our fine-grained OSR experiments. 
The drawback of such a method is that the concept of `similarity' between classes is abstractly conditioned on the training data of the feature embedding. 
Ideally, the concept of similarity would be `objectively' (\ie~in a human interpretable fashion) related to the semantic axis of variation which we wish the OSR model to learn. 
It is for this reason that we use labelled attributes to create the splits.
We believe there could be multiple valid ways for creating the splits for OSR, which we leave as future work.

Furthermore, we show in the main paper that the performance of current OSR models in the new setting is far from saturated. 
However, the proposed FGVC setting opens the door to a number of methods which were previously infeasible. 
For instance, models which learn attributes for each training class may perform better. 
Images from novel classes could then be identified if they share few attributes with the training classes.

\paragraph{Ethical considerations}
Open-set recognition is of immediate relevance to the safe and ethical deployment of machine learning models. 
In real-world settings, it is unrealistic to expect that all categories of interest to the user will be represented in the training set. 
For instance, in an autonomous driving scenario, forcing the model to identify every object as an instance of a training category could lead it to make unsafe decisions.

When considering potential negative societal impacts of this work, we identify the possibility that OSR research may lead to complacent consideration of the training data. 
As we have demonstrated, OSR models are far from perfect and cannot be exclusively relied upon in practical deployment.
As such, it remains of critical importance to carefully curate training data and ensure its distribution is representative of the target task.
